# Supplementary material for: HyperColorization: Propagating spatially sparse noisy spectral clues for reconstructing hyperspectral images
Source: arXiv:2403.11935 source file (2024-03-18)
Supplement: Supplementary file 1 [file supplement.pdf]

# HYPERCOLORIZATION: PROPAGATING SPATIALLY SPARSE NOISY SPECTRAL CLUES OVER HYPERPECTRAL IMAGES: SUPPLEMENTAL DOCUMENT

## HyperColorization Rank and Exposure Time: Additional Examples

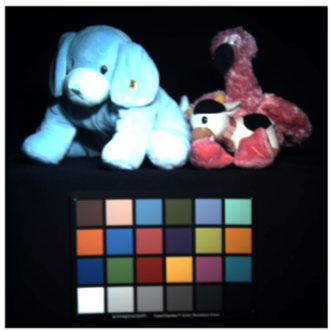

(a)

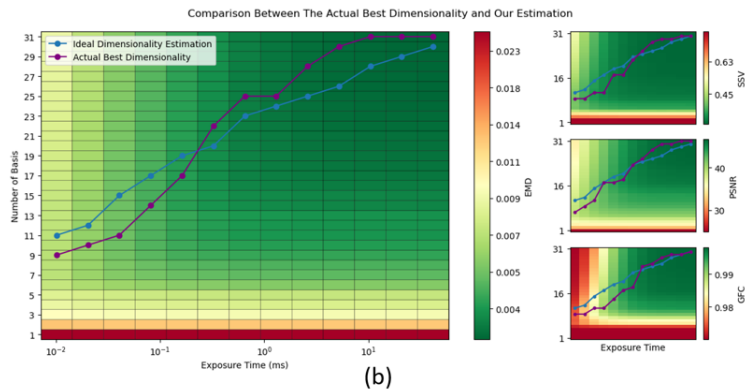

(b)

Figure S1. Image from CAVE dataset [1], brightness boosted by 20%. (b) How the optimal and estimated colorization dimensionality varies with exposure time for image in (a).

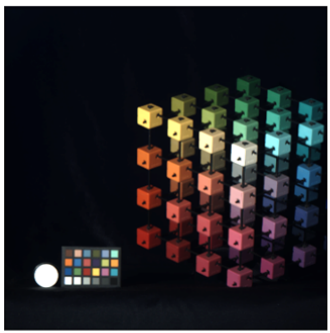

(a)

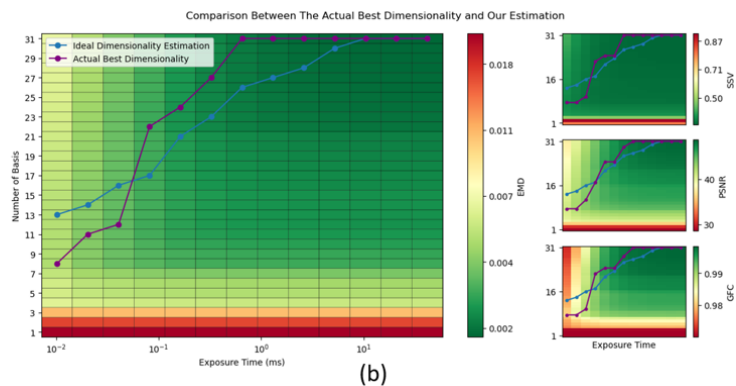

(b)

Figure S2 Image from KAIST dataset [4], brightness boosted by 40%. (b) How the optimal and estimated colorization dimensionality varies with exposure time for image in (a).

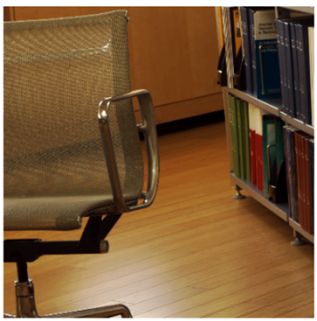

(a)

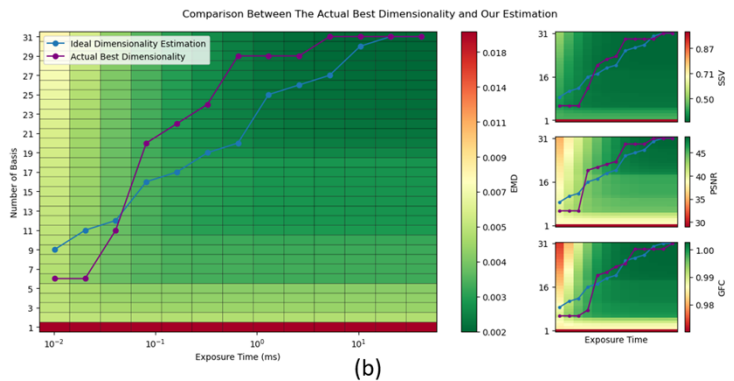

(b)

Figure S3 Image from Harvard dataset [2], brightness boosted by 65%. (b) How the optimal and estimated colorization dimensionality varies with exposure time for image in (a).

## Sampling Patterns: Additional Examples

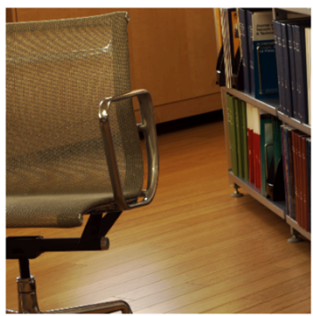

Ground Truth

Push Broom

Sampling Ratio: 5%

Whisk Broom

Sampling Ratio: 0.5%

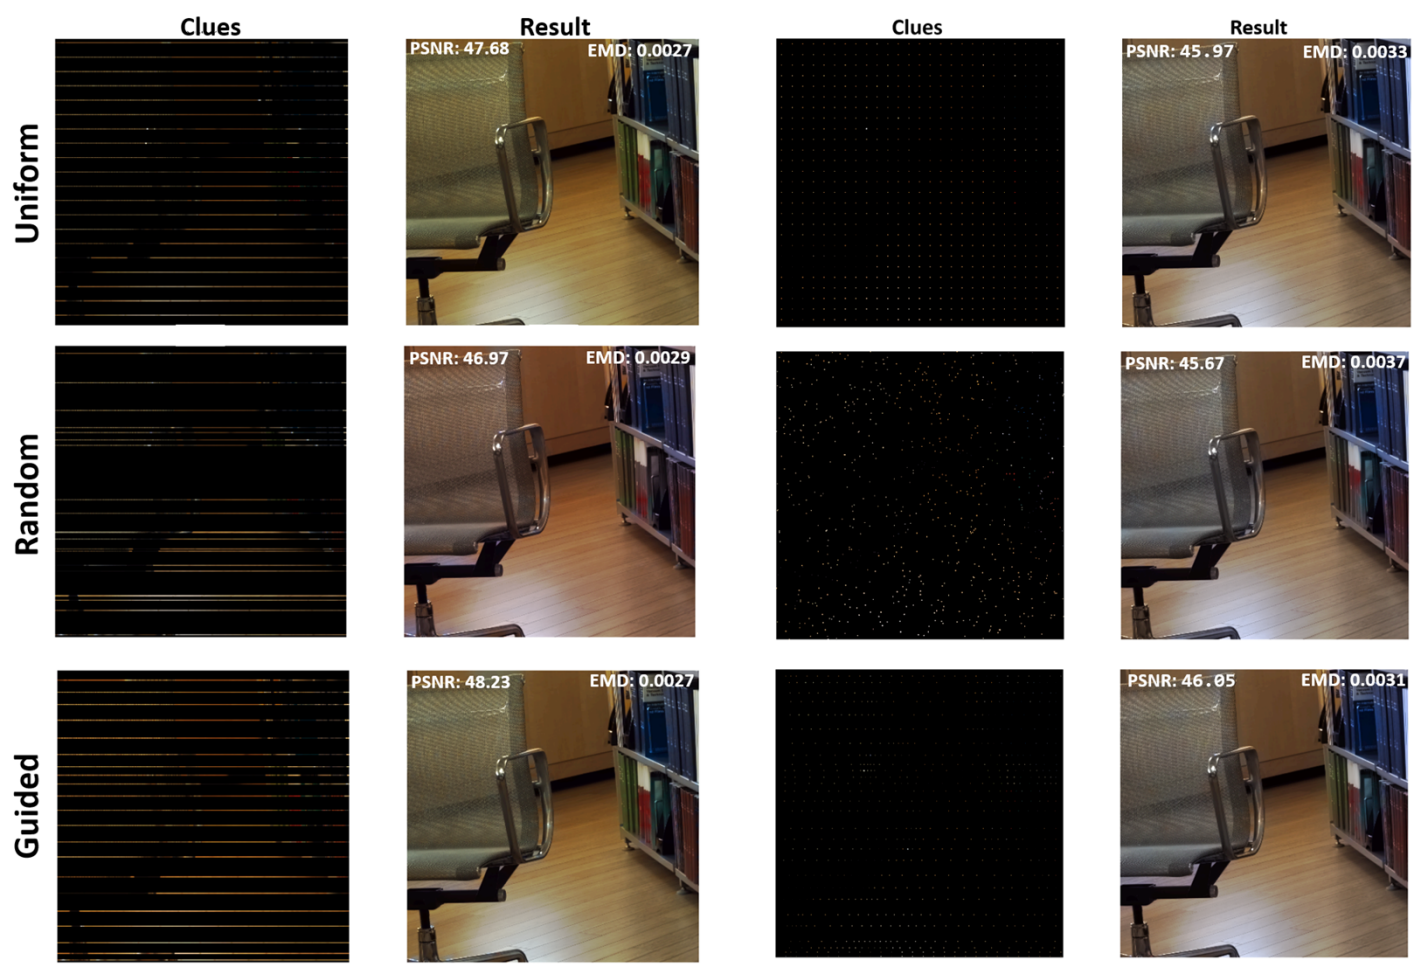

Figure S4. Brightness is boosted by 65% and size of spectral clues increased. Image from the Harvard dataset [2].

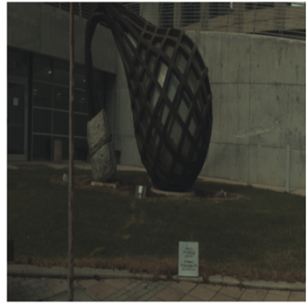

Ground Truth

Push Broom

Whisk Broom

Sampling Ratio: 10%

Sampling Ratio: 1%

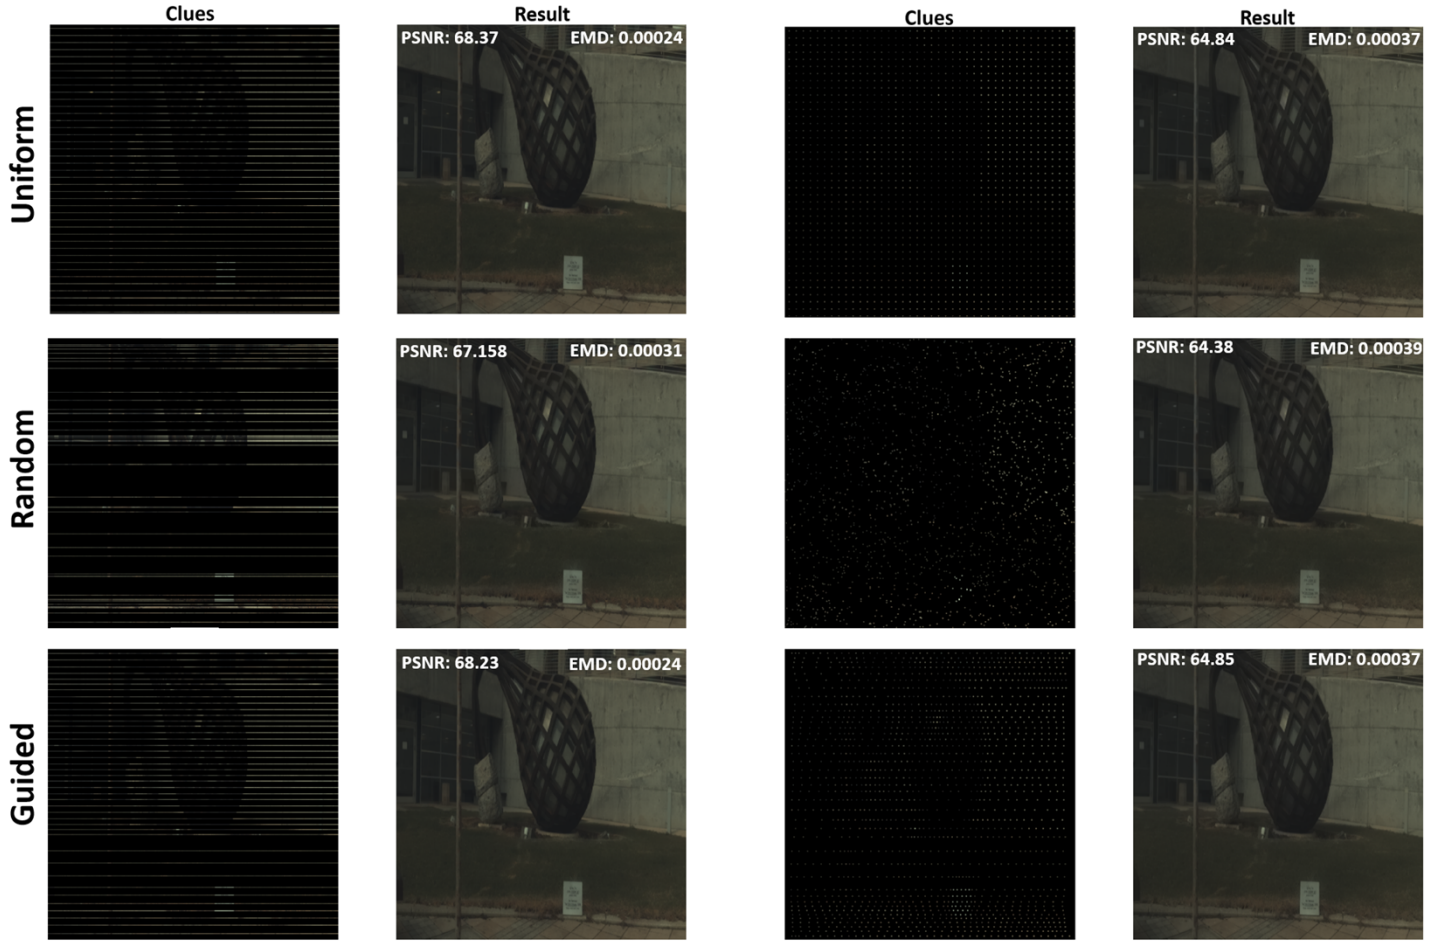

Figure S5. Brightness boosted by 30% and size of spectral clues increased. Image from the ICVL dataset [3] which features 512 channels.

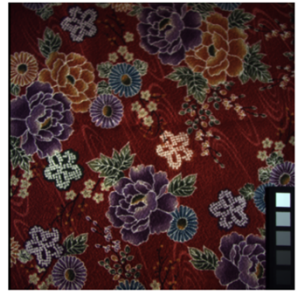

Ground Truth

Push Broom

Whisk Broom

Sampling Ratio: 10%

Sampling Ratio: 1%

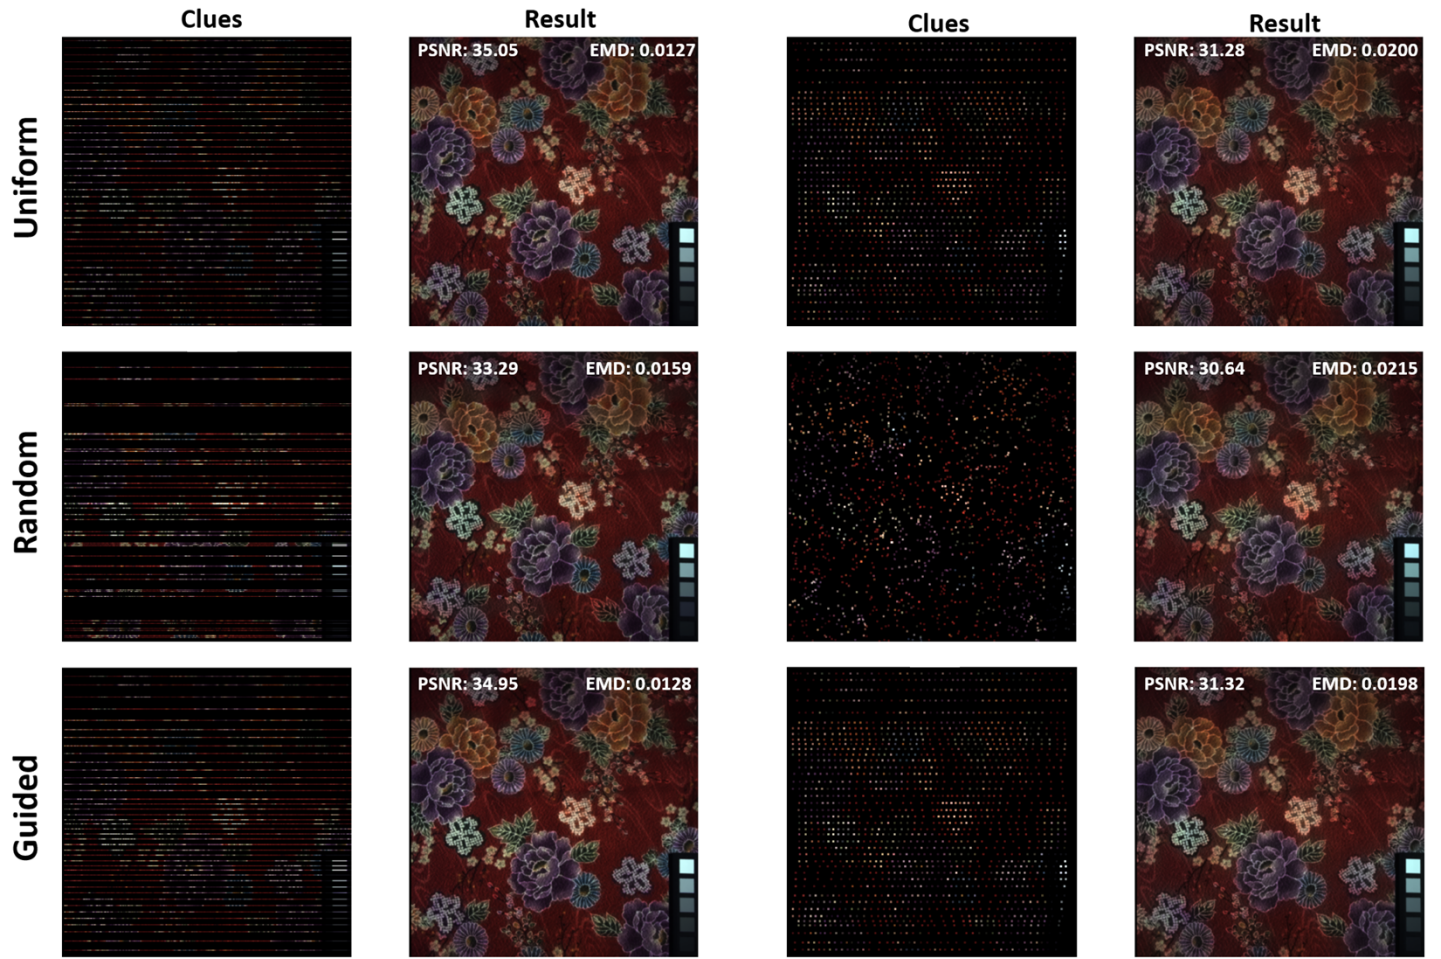

Figure S6. Brightness boosted by 40% and size of spectral clues increased. Image from the CAVE dataset [1] where guided sampling is outperformed by uniform sampling.

## Imaging with a Fixed Time Budget: Additional Examples

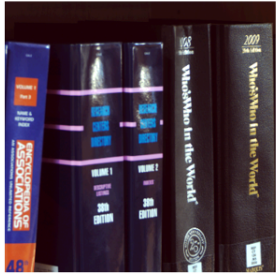

(a)

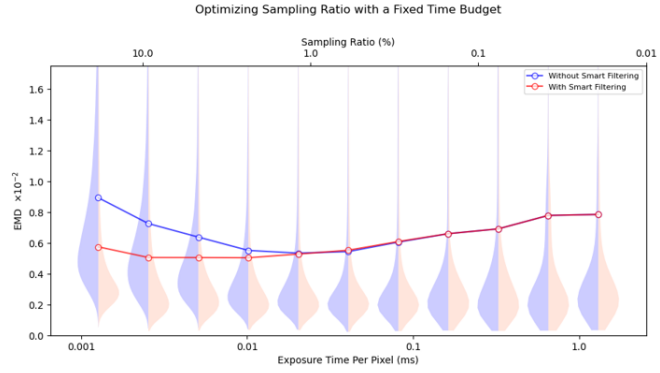

(b)

Figure S7 (a) Image from Harvard dataset [2], brightness boosted by 70%. (b) The trade-off between sampling ratio and exposure time when smart filter is enabled and disabled on image (a).

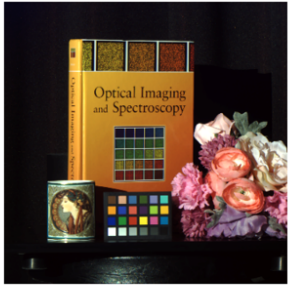

(a)

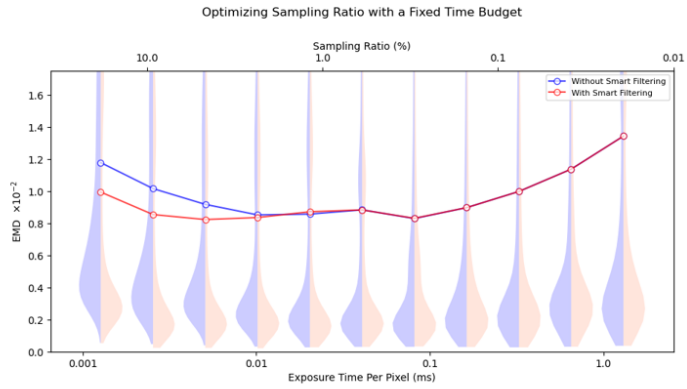

(b)

Figure S8 (a) Image from KAIST dataset [4], brightness boosted by 50%. (b) The trade-off between sampling ratio and exposure time when smart filter is enabled and disabled on image (a).

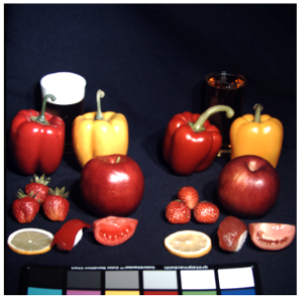

(a)

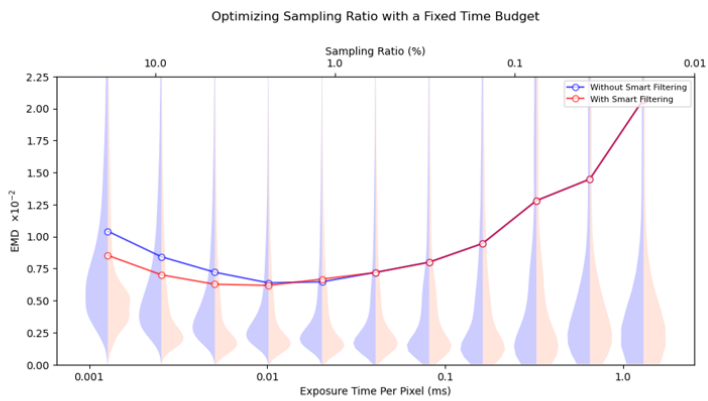

(b)

Figure S9 (a) Image from CAVE dataset [1], brightness boosted by 60%. (b) The trade-off between sampling ratio and exposure time when smart filter is enabled and disabled on image (a).

**Table S1. Sampling Patterns Performance Analysis on Harvard dataset**

| Sampling Type       | Sampling Ratio | PSNR↑  | SSV↓  | GFC↑  | EMD ↓ $10^{-3}$ |
|---------------------|----------------|--------|-------|-------|-----------------|
| Uniform push broom  | 10%            | 37.938 | 0.342 | 0.992 | 6.865           |
| Uniform push broom  | 4%             | 35.155 | 0.433 | 0.989 | 9.340           |
| Guided push broom   | 4%             | 35.500 | 0.409 | 0.989 | 9.261           |
| Uniform whisk broom | 4%             | 37.895 | 0.358 | 0.992 | 6.789           |
| Guided whisk broom  | 4%             | 38.457 | 0.352 | 0.992 | 6.607           |
| Uniform whisk broom | 1%             | 36.290 | 0.416 | 0.990 | 8.881           |
| Guided whisk broom  | 1%             | 36.597 | 0.413 | 0.989 | 7.853           |

## References

1. F. Yasuma, T. Mitsunaga, D. Iso, and S. K. Nayar, "Generalized Assorted Pixel Camera: Postcapture Control of Resolution, Dynamic Range, and Spectrum," *IEEE Transactions on Image Processing* 19(9), 2241–2253 (2010).
2. A. Chakrabarti and T. Zickler, "Statistics of real-world hyperspectral images," in *CVPR 2011* (2011), pp. 193–200.
3. B. Arad and O. Ben-Shahar, "Sparse Recovery of Hyperspectral Signal from Natural RGB Images," in *European Conference on Computer Vision* (Springer, 2016), pp. 19–34.
4. I. Choi, D. S. Jeon, G. Nam, D. Gutierrez, and M. H. Kim, "High-Quality Hyperspectral Reconstruction Using a Spectral Prior," *ACM Transactions on Graphics (Proc. SIGGRAPH Asia 2017)* 36(6), 218:1–13 (2017).
5. X. Cao, X. Tong, Q. Dai, and S. Lin, "High resolution multispectral video capture with a hybrid camera system," in *CVPR 2011* (2011), pp. 297–304.
6. V. Saragadam and A. C. Sankaranarayanan, "KRISM—Krylov Subspace-based Optical Computing of Hyperspectral Images," *ACM Trans. Graph.* 38(5), 1–14 (2019).
